# Supplementary material for: Meta-Learning Regrasping Strategies for Physical-Agnostic Objects
Source: arXiv:2205.11110 source file (2023-09-14)
Supplement: Supplementary file 1 [file appendix.tex]

\subsection{Typical Failure Scenario}
\begin{figure}[H]
	\centering
	\hfill
	\begin{subfigure}[htbp]{0.33\textwidth}
		\centering
		\includegraphics[width=1\textwidth]{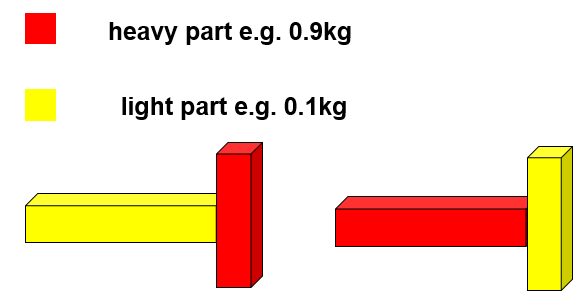}
		\caption{Two hammer-shaped objects}
		\label{fig:two-hammer-shaped-objects}
	\end{subfigure}
	\hfill
	\begin{subfigure}[htbp]{0.10\textwidth}
		\centering
		\includegraphics[width=1\textwidth]{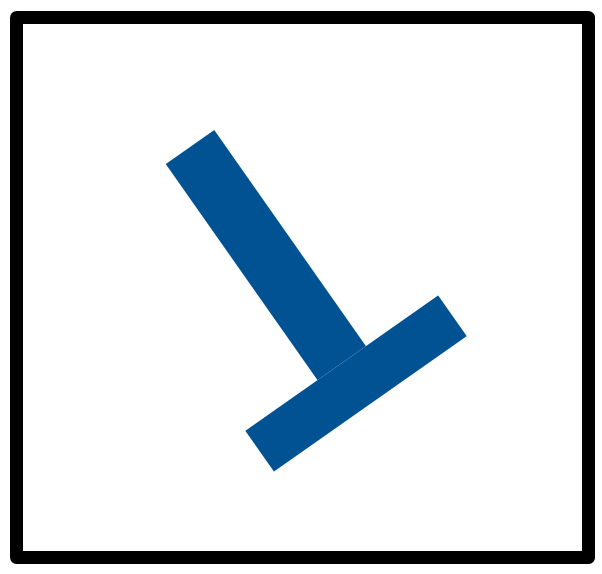}
		\caption{Perceived visual input}
		\label{fig:visual-perception}
	\end{subfigure}
	\caption{\textbf{Typical failure scenario for visual-based methods. }Two objects have the same geometry, texture, and size except for mass distribution. The perceived visual information for visual-based grasp detection algorithms is therefore the same, resulting in detection failure.}
	\label{fig:typical-failure-scenario}
\end{figure}

\subsection{Object Datasets}

\begin{table}[H]%
	\centering%
	\begin{tabular}{lll}
		\toprule
		Object Variant & Total Weight & Cube Size\\
		\midrule
		Letter F & 1kg & (0.027, 0.033)\\
		Letter L & 1kg & (0.027, 0.033)\\
		Letter T & 1kg & (0.027, 0.033)\\
		Number Four & 1kg & (0.027, 0.033)\\
		Number Nine & 1kg & (0.027, 0.033)\\
		\bottomrule
	\end{tabular}
	\caption{\textbf{Configuration overview of different shape categories. }The total object weight in each shape category is set to be 1kg and the cube size ranges continuously from 2.7~cm to 3.3~cm.}
	\label{tab:configuration-overview}%
\end{table}

\begin{figure}[H]
	\centering
	\includegraphics[width=0.20\textwidth]{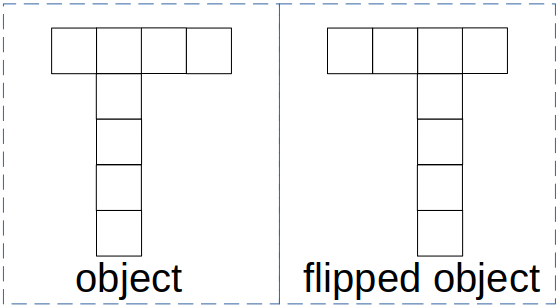}
	\caption{\textbf{Exemplary image of flip operation. }We use flip augmentation to increase object dataset size.}
	\label{fig:flip-object}%
\end{figure}%

\subsection{GQ-CNN-CNP Network Architecture Detail}

\begin{figure}[H]
	\centering
	
	\begin{subfigure}[htbp]{0.46\textwidth}
		\centering
		\includegraphics[width=1\textwidth]{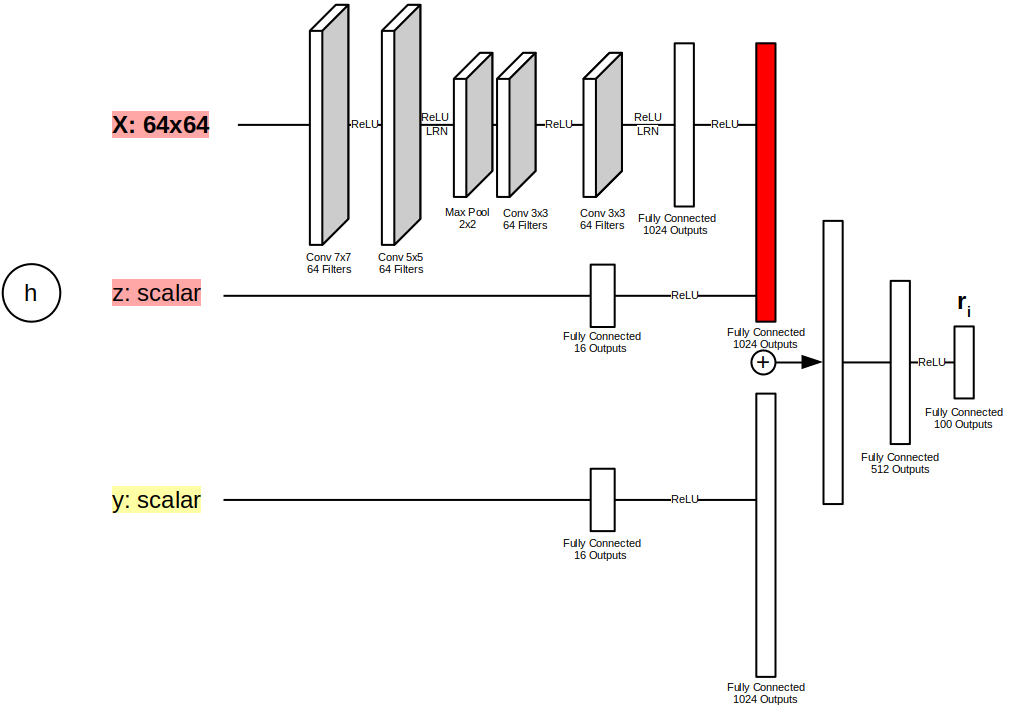}
		\caption{encoder part of GQ-CNN-CNP}
		\label{fig:CNP-encoder}
	\end{subfigure}
	\vfill
	\begin{subfigure}[htbp]{0.49\textwidth}
		\centering
		\includegraphics[width=1\textwidth]{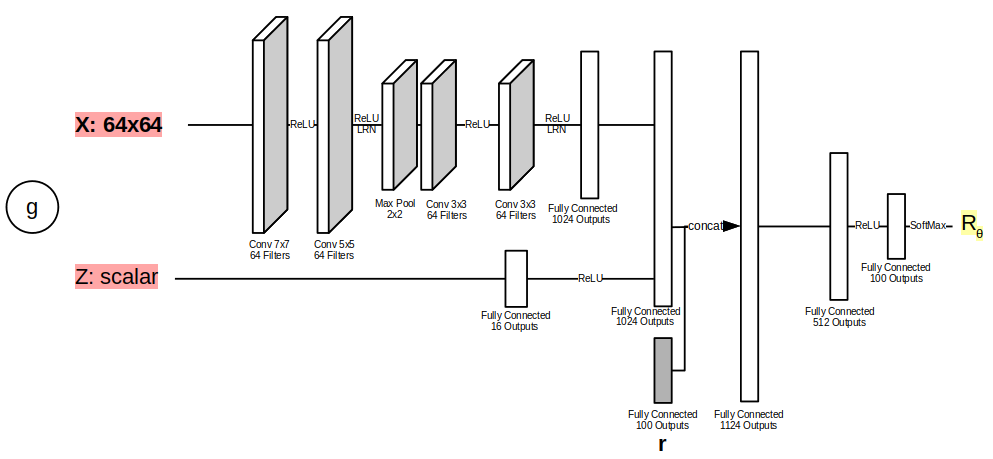}
		\caption{decoder part of GQ-CNN-CNP}
		\label{fig:CNP-decoder}
	\end{subfigure}
	\vfill
	\begin{subfigure}[htbp]{0.18\textwidth}
		\centering
		\includegraphics[width=1\textwidth]{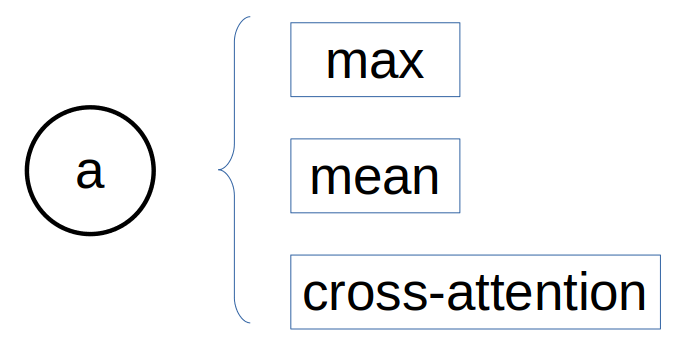}
		\caption{aggregation method}
		\label{fig:aggregation-overview}
	\end{subfigure}
	\caption{\textbf{GQ-CNN-CNP implementation. }h stands for the encoder that extracts object representation from context observations. g stands for the decoder that predicts grasping robustness on target grasping candidates. a can be any form of aggregators gathering the extracted context information.}
	\label{fig:GQCNN-CNP-architecture-detail}
\end{figure}

\subsection{Statistics of Collected Image Data}
\begin{figure}[H]
	\centering
	\includegraphics[width=0.35\textwidth]{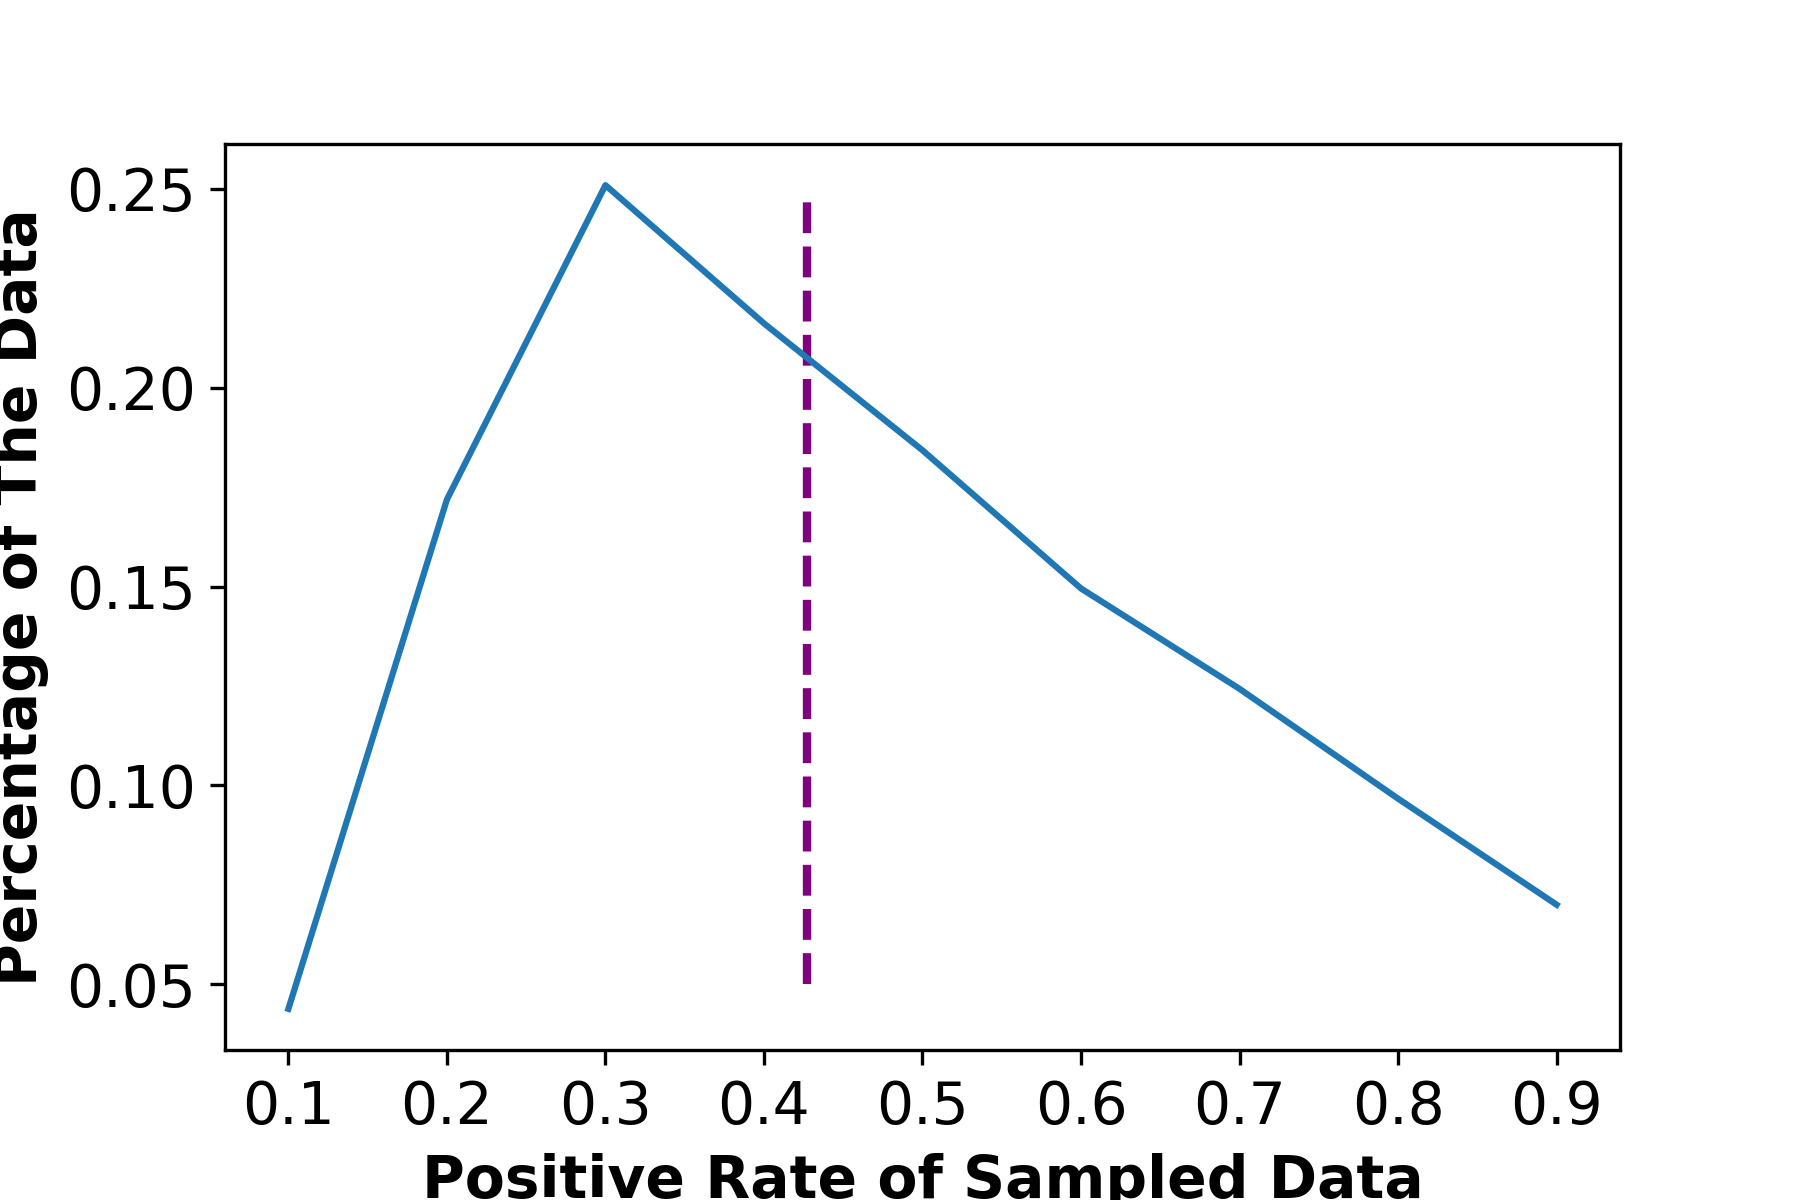}
	\caption{\textbf{Relative frequency distribution of grasping positive rate of across all 10 shape categories.} The purple dashed line indicates the average positive rate of 42.7\%.}
	\label{fig:overall-positive-rate}
\end{figure}

\subsection{Experiment on Meta-learning Classification Task}

\begin{table}[H]%
	\centering%
	\begin{tabular}{lll}
		\toprule
		Model Variant & Task Augmentation & Context Size\\
		\midrule
		GQ-CNN-CNP-att-10con & None & [10, 15]\\
		GQ-CNN-CNP-att-aug-10con & Yes & [10, 15]\\
		GQ-CNN-CNP-att-aug-1con & Yes & [1, 15]\\
		GQ-CNN & None & None\\
		\bottomrule
	\end{tabular}
	\caption{\textbf{Overview of model variants. }None is marked when the case is not applicable. In the training stage, context size is randomly selected from a given interval for each episode.}
	\label{tab:network-variant-overview}%
\end{table}

\begin{figure}[H]
	\centering
	\includegraphics[width=0.49\textwidth]{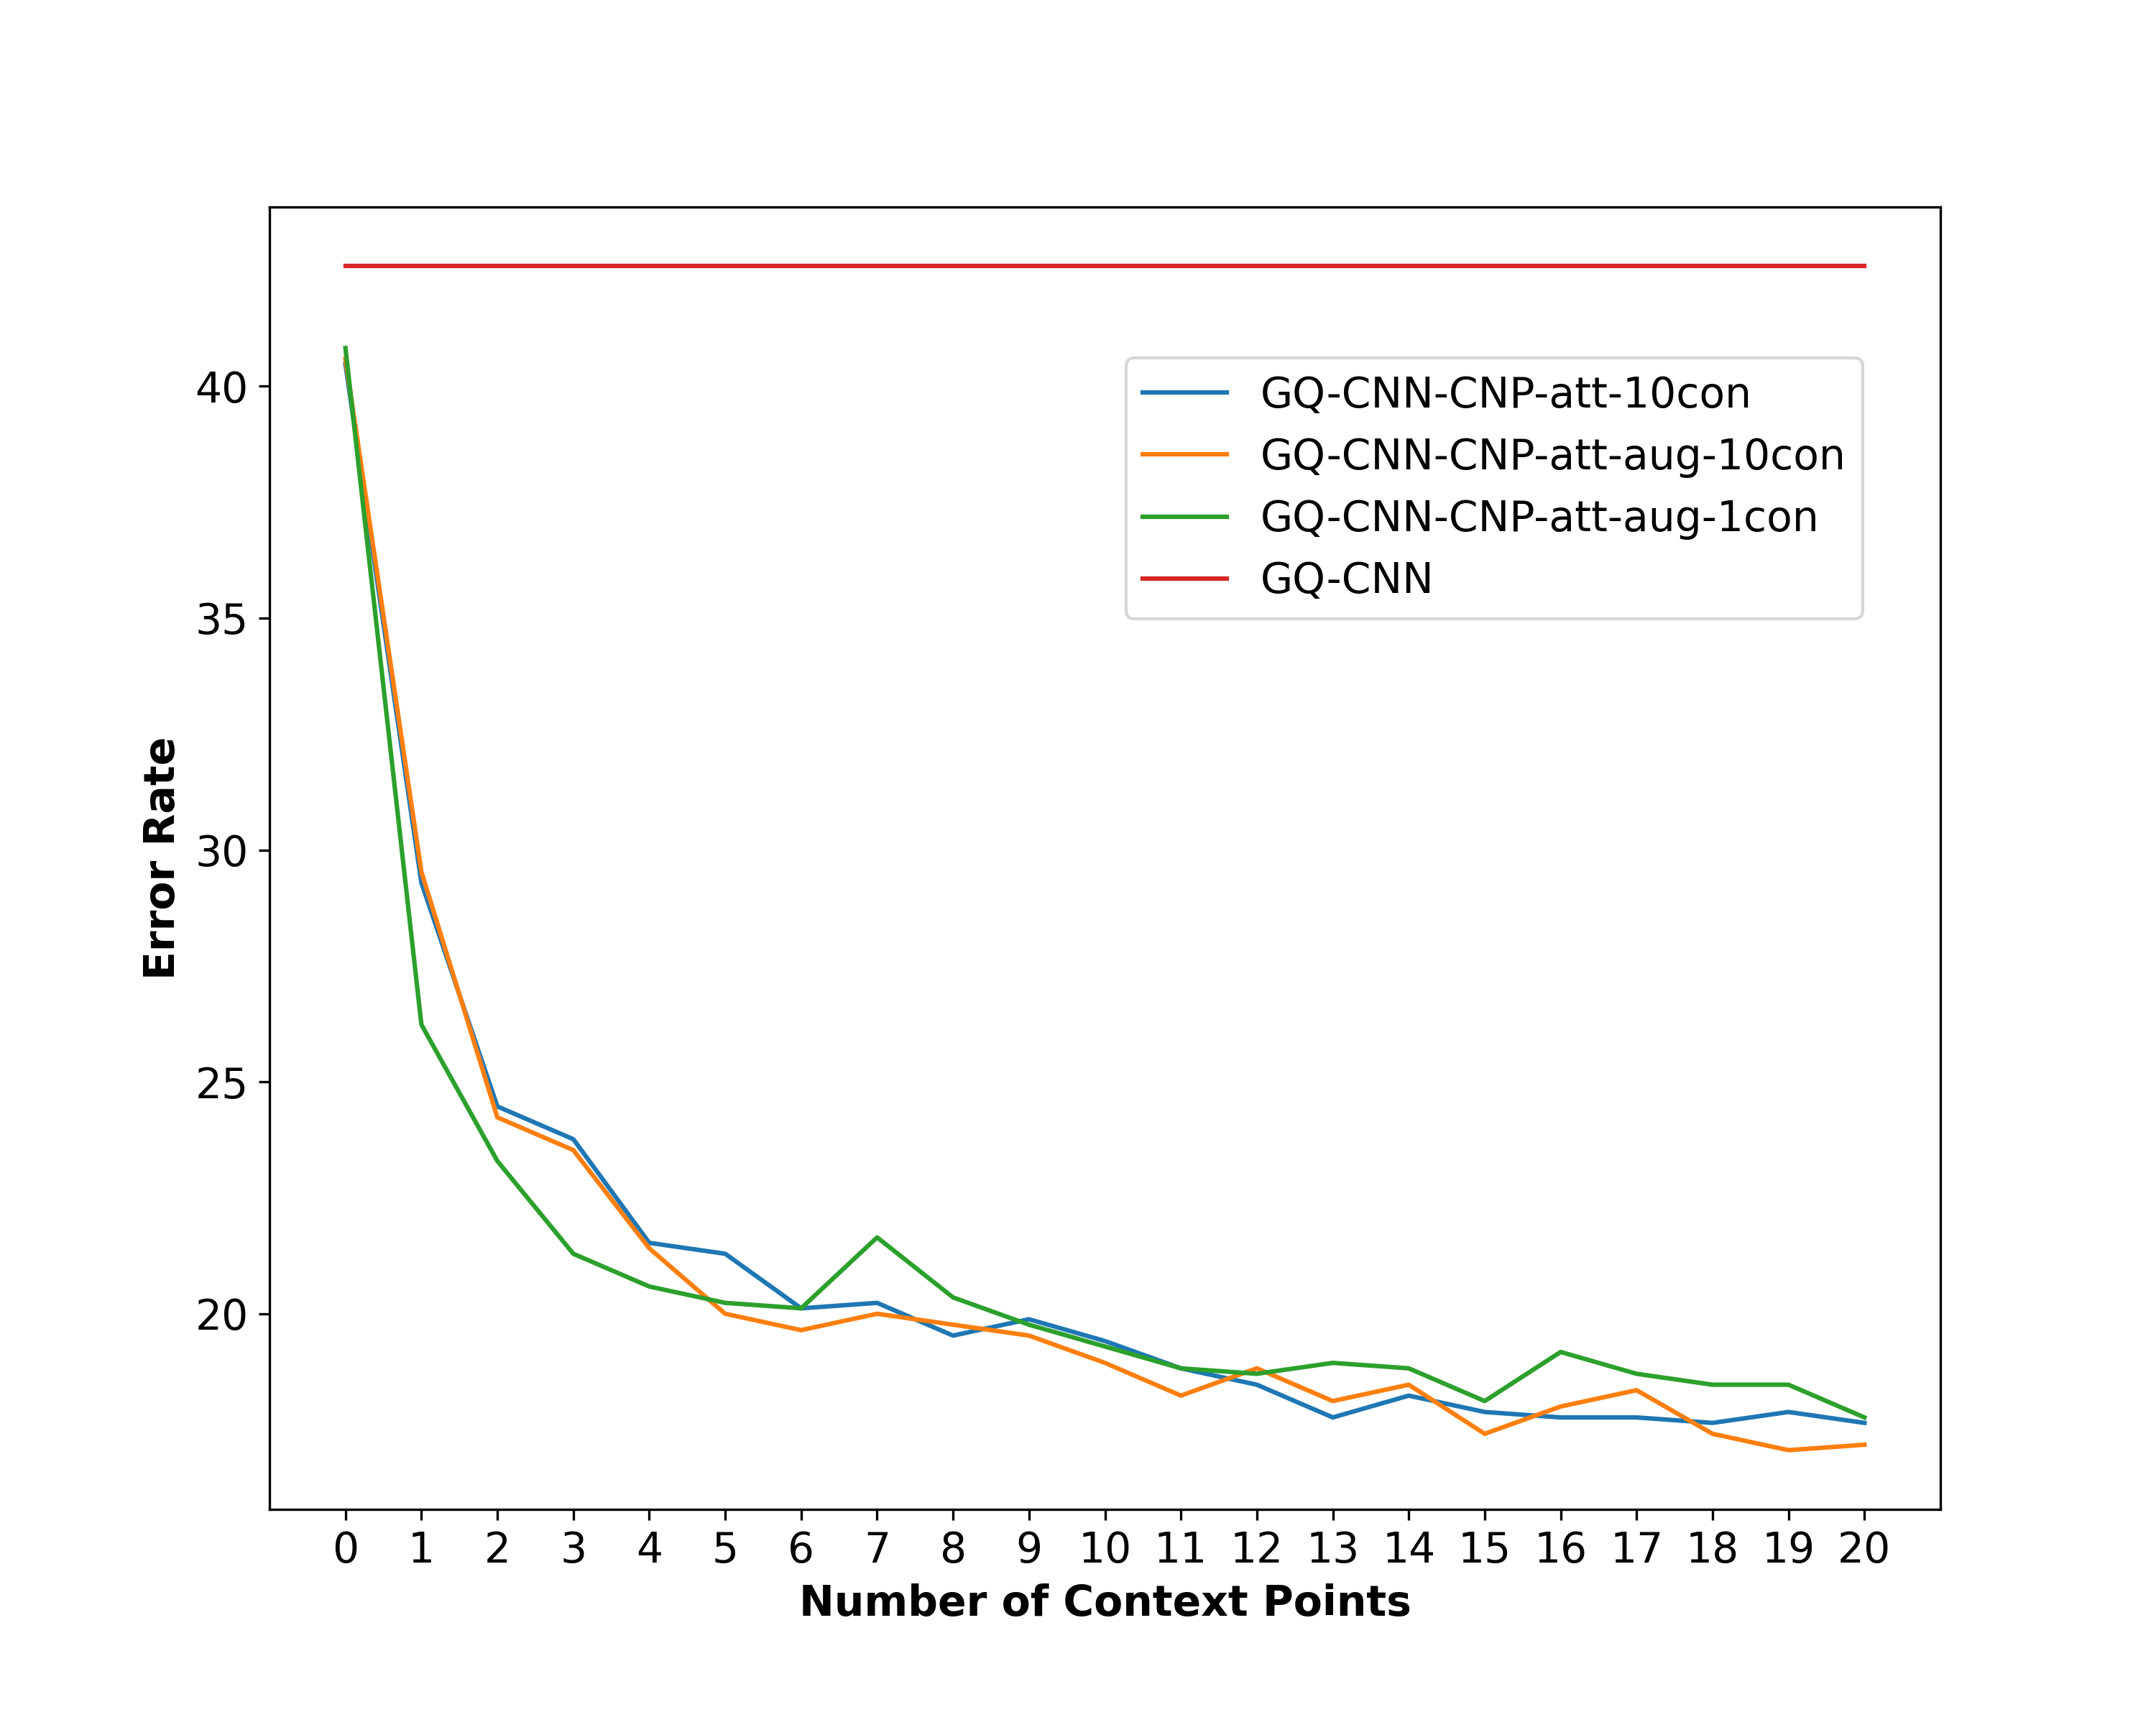}
	\caption{\textbf{Error rate vs number of context points on intra-category objects. }Curves indicate the error rate of robustness prediction across different model variants, based on 83 object instances from the 8 intra-categories.}
	\label{fig:validation-set-error-rate-appendix}
\end{figure}

\begin{figure}[H]
	\centering
	\includegraphics[width=0.49\textwidth]{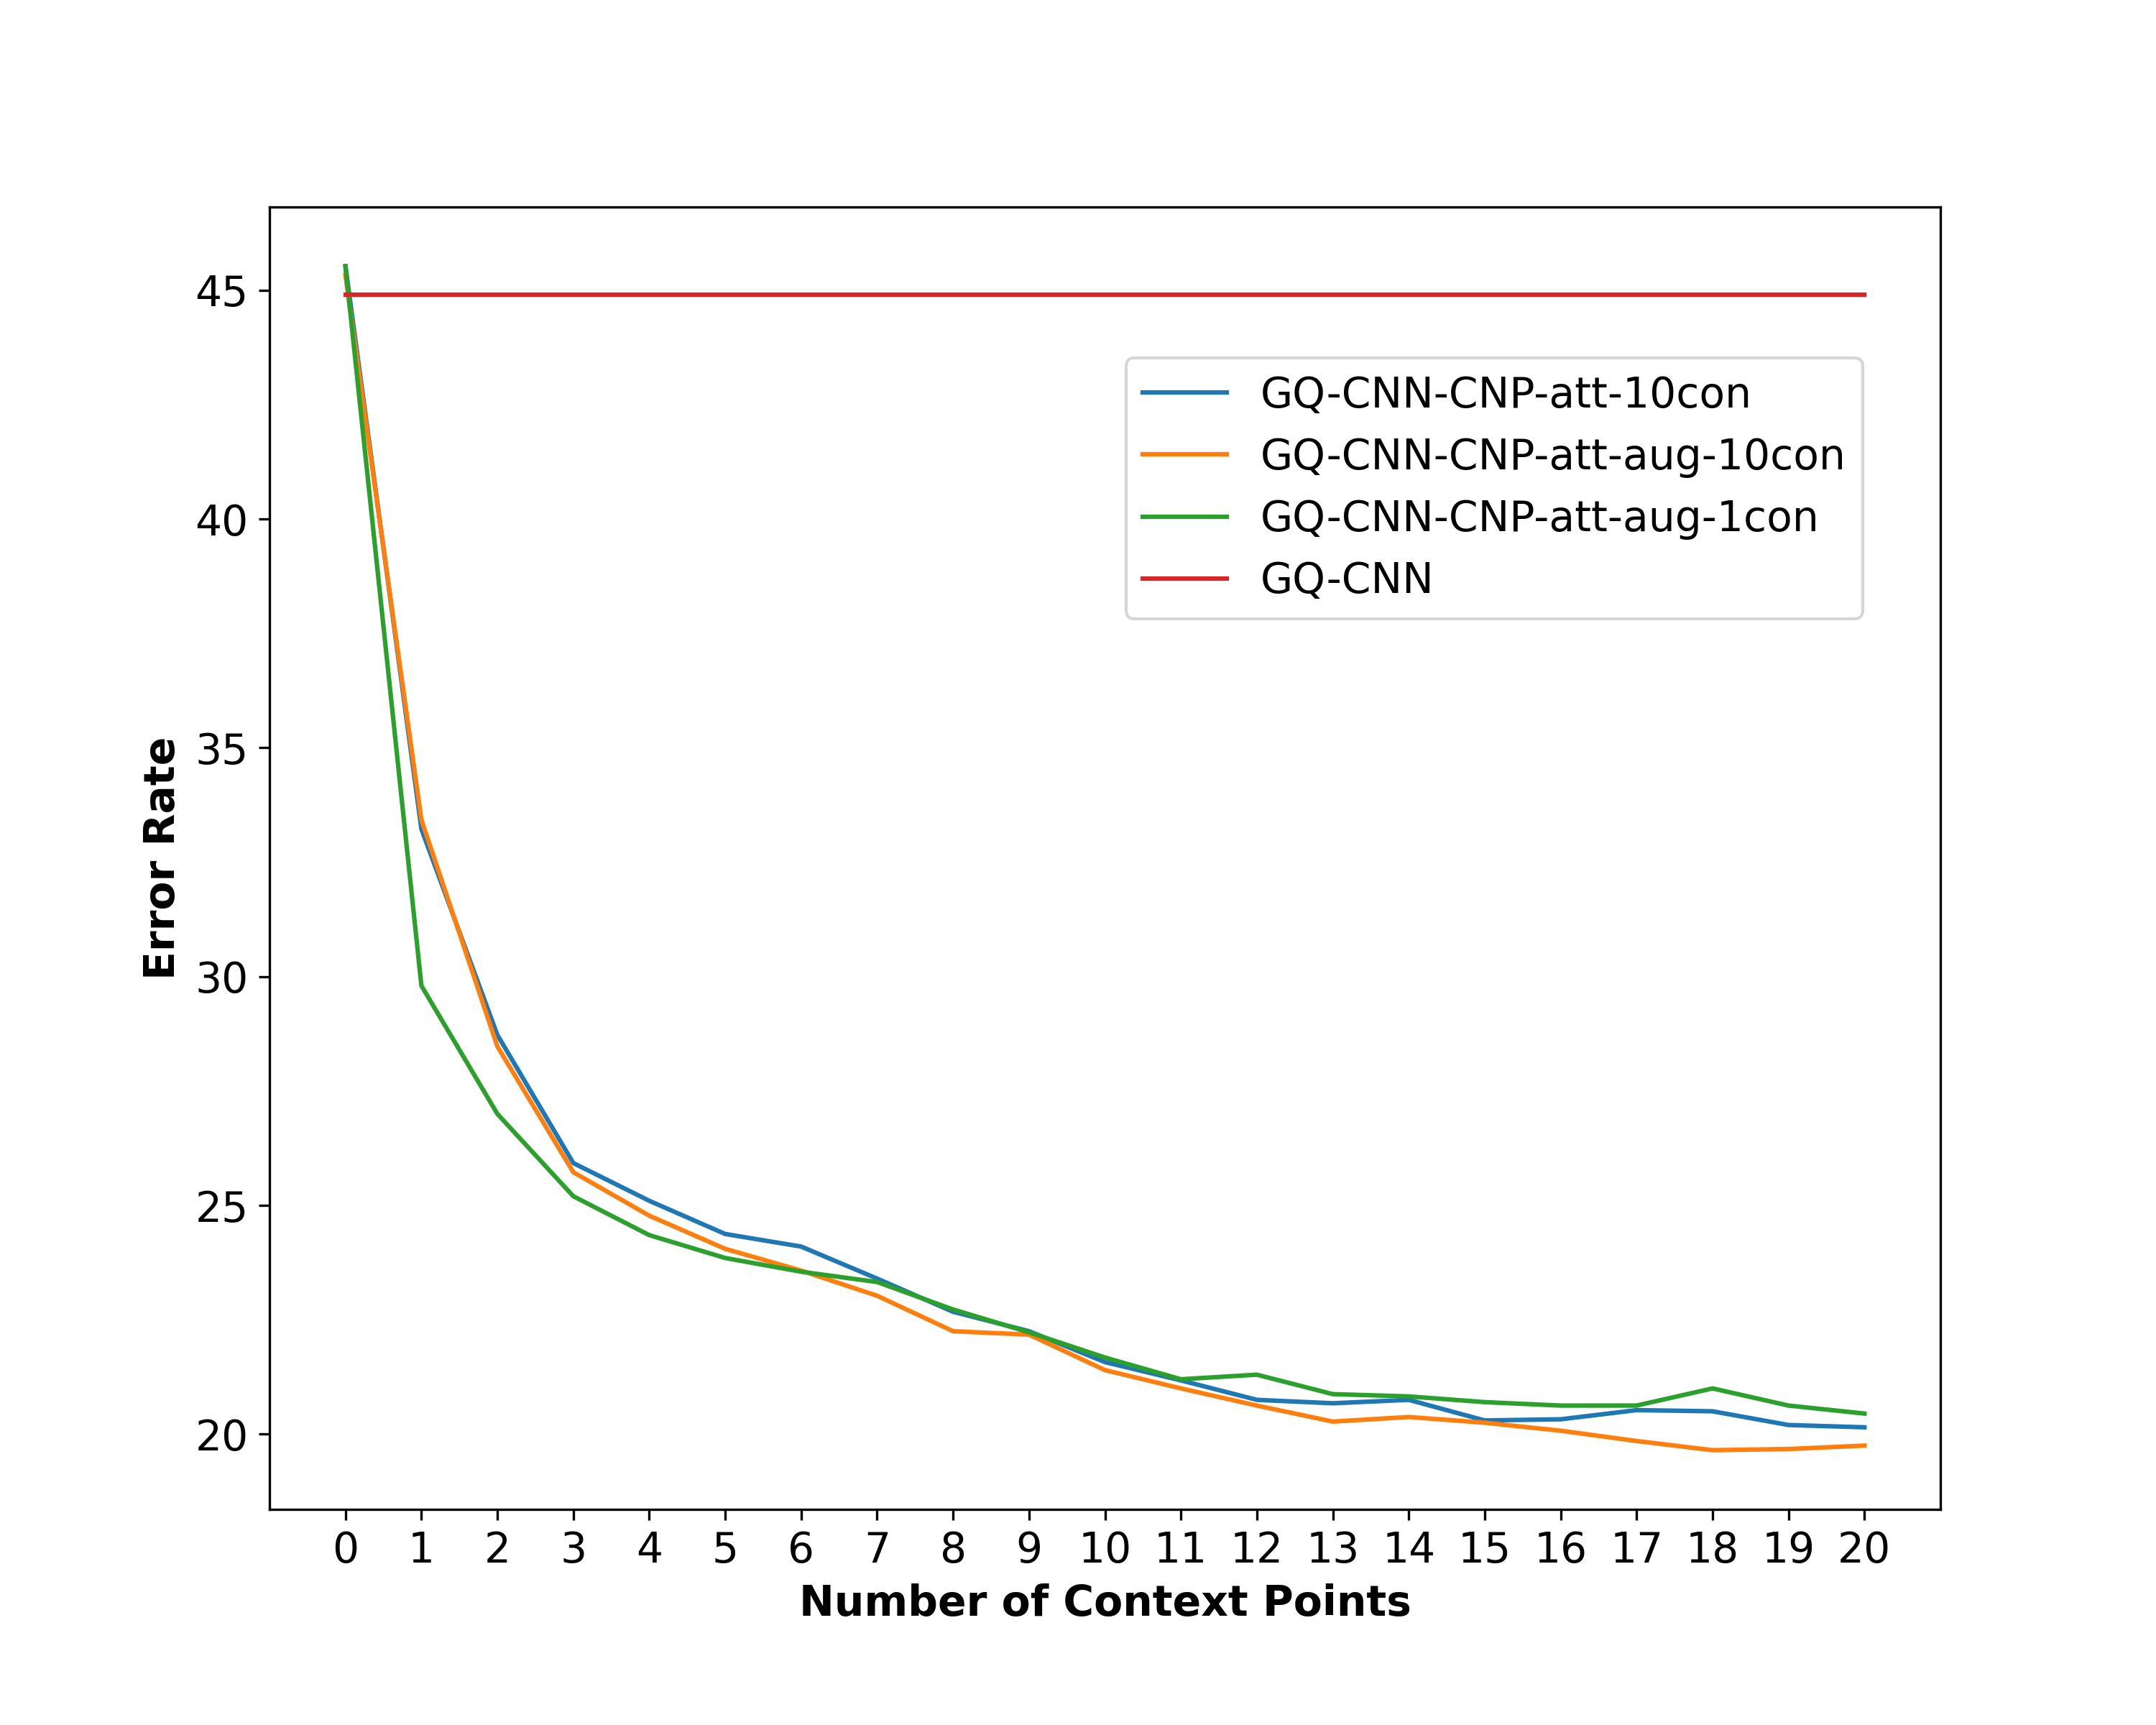}
	\caption{\textbf{Error rate vs number of context points on cross-category objects. }Curves indicate the error rate of robustness prediction across different model variants, based on 450 object instances from the 2 cross-categories.}
	\label{fig:test-set-error-rate-appendix}
\end{figure}

Four network variants (see Tab.~\ref{tab:network-variant-overview}) are evaluated on both intra-category (IC) and cross-category (CC) objects. The results are shown above in Fig.~\ref{fig:validation-set-error-rate-appendix} and Fig.~\ref{fig:test-set-error-rate-appendix}.

\subsection{Side Experiments on Grasping Benchmark}

\textbf{Robust Grasping Rate.} The percentage of planned grasps with estimated robustness higher than 50\%, is another metric for grasping benchmark in addition to grasping success rate.

Fig.~\ref{fig:label-positive-rate-comparison} shows a difference in the positive rate of collected context points between 2 mechanisms, DexNet-CNP-ACC and DexNet-CNP-Once. DexNet-CNP-ACC is much higher than DexNet-CNP-Once. Consistent with our expectation, DexNet-CNP-ACC results in a higher robust grasping rate due to an overconfidence in prediction (see Fig.~\ref{fig:robust-rate-comparison}). However, a higher positive rate in collected context observations doesn't necessarily improve the grasping success rate (see Fig.~\ref{fig:grasping-success-comparison(sampling strategy)}).

We further vary the size of cropped depth image, $64 \times 64$ (object fully visible) and $32 \times 32$ (object partially visible). The benchmark performance is better with larger image size (see Fig.~\ref{fig:grasping-success-comparison(field of view)}), based on which we assume that the model can better reason about physical properties with the full view of an object.

\begin{figure}[H]
	\centering
	\includegraphics[width=0.30\textwidth]{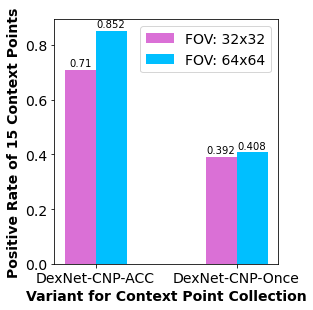}
	\caption{\textbf{Comparison of label's positive rate. }The context positive rate for each mechanism based on 50 object instances from intra- and cross-categories is indicated. Two fields of view (FOVs) are shown in different colors.}
	\label{fig:label-positive-rate-comparison}
\end{figure}

\begin{figure}[H]
	\centering
	\includegraphics[width=0.49\textwidth]{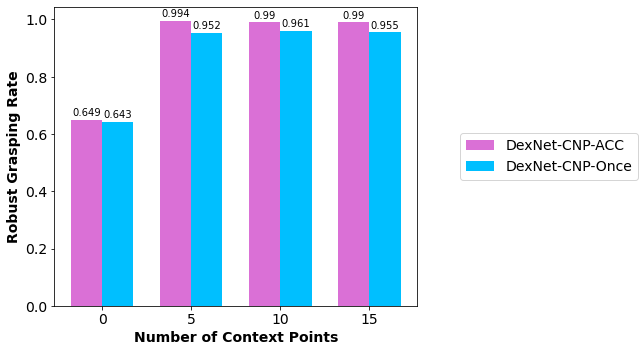}
	\caption{\textbf{Comparison of robust grasping rate. }The robust grasping rate w.r.t two context collection mechanisms is plotted.}
	\label{fig:robust-rate-comparison}
\end{figure}

\begin{figure}[htbp]
	\centering
	\includegraphics[width=0.49\textwidth]{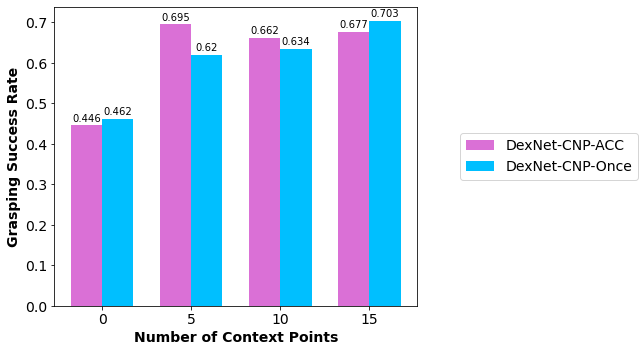}
	\caption{\textbf{Comparison of grasping success rate. }The grasping success rate w.r.t two context collection mechanisms is plotted.}
	\label{fig:grasping-success-comparison(sampling strategy)}
\end{figure}

\begin{figure}[htbp]
	\centering
	\includegraphics[width=0.44\textwidth]{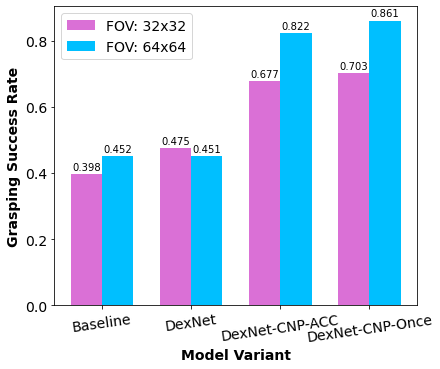}
	\caption{\textbf{Comparison of grasping success rate. }The grasping success rate of each field of view is plotted across model variants.}
	\label{fig:grasping-success-comparison(field of view)}
\end{figure}
